# Supplementary material for: A parameter-free mechanistic model of the adhesive wear process of rough surfaces in sliding contact
Source: arXiv:2004.00559 source file (2021-01-19)
Supplement: Supplementary file 1 [file supplementary.pdf]

*Supplementary Data*

# A parameter-free mechanistic model of the adhesive wear process of rough surfaces in sliding contact

Tobias Brink, Lucas Frérot, and Jean-François Molinari

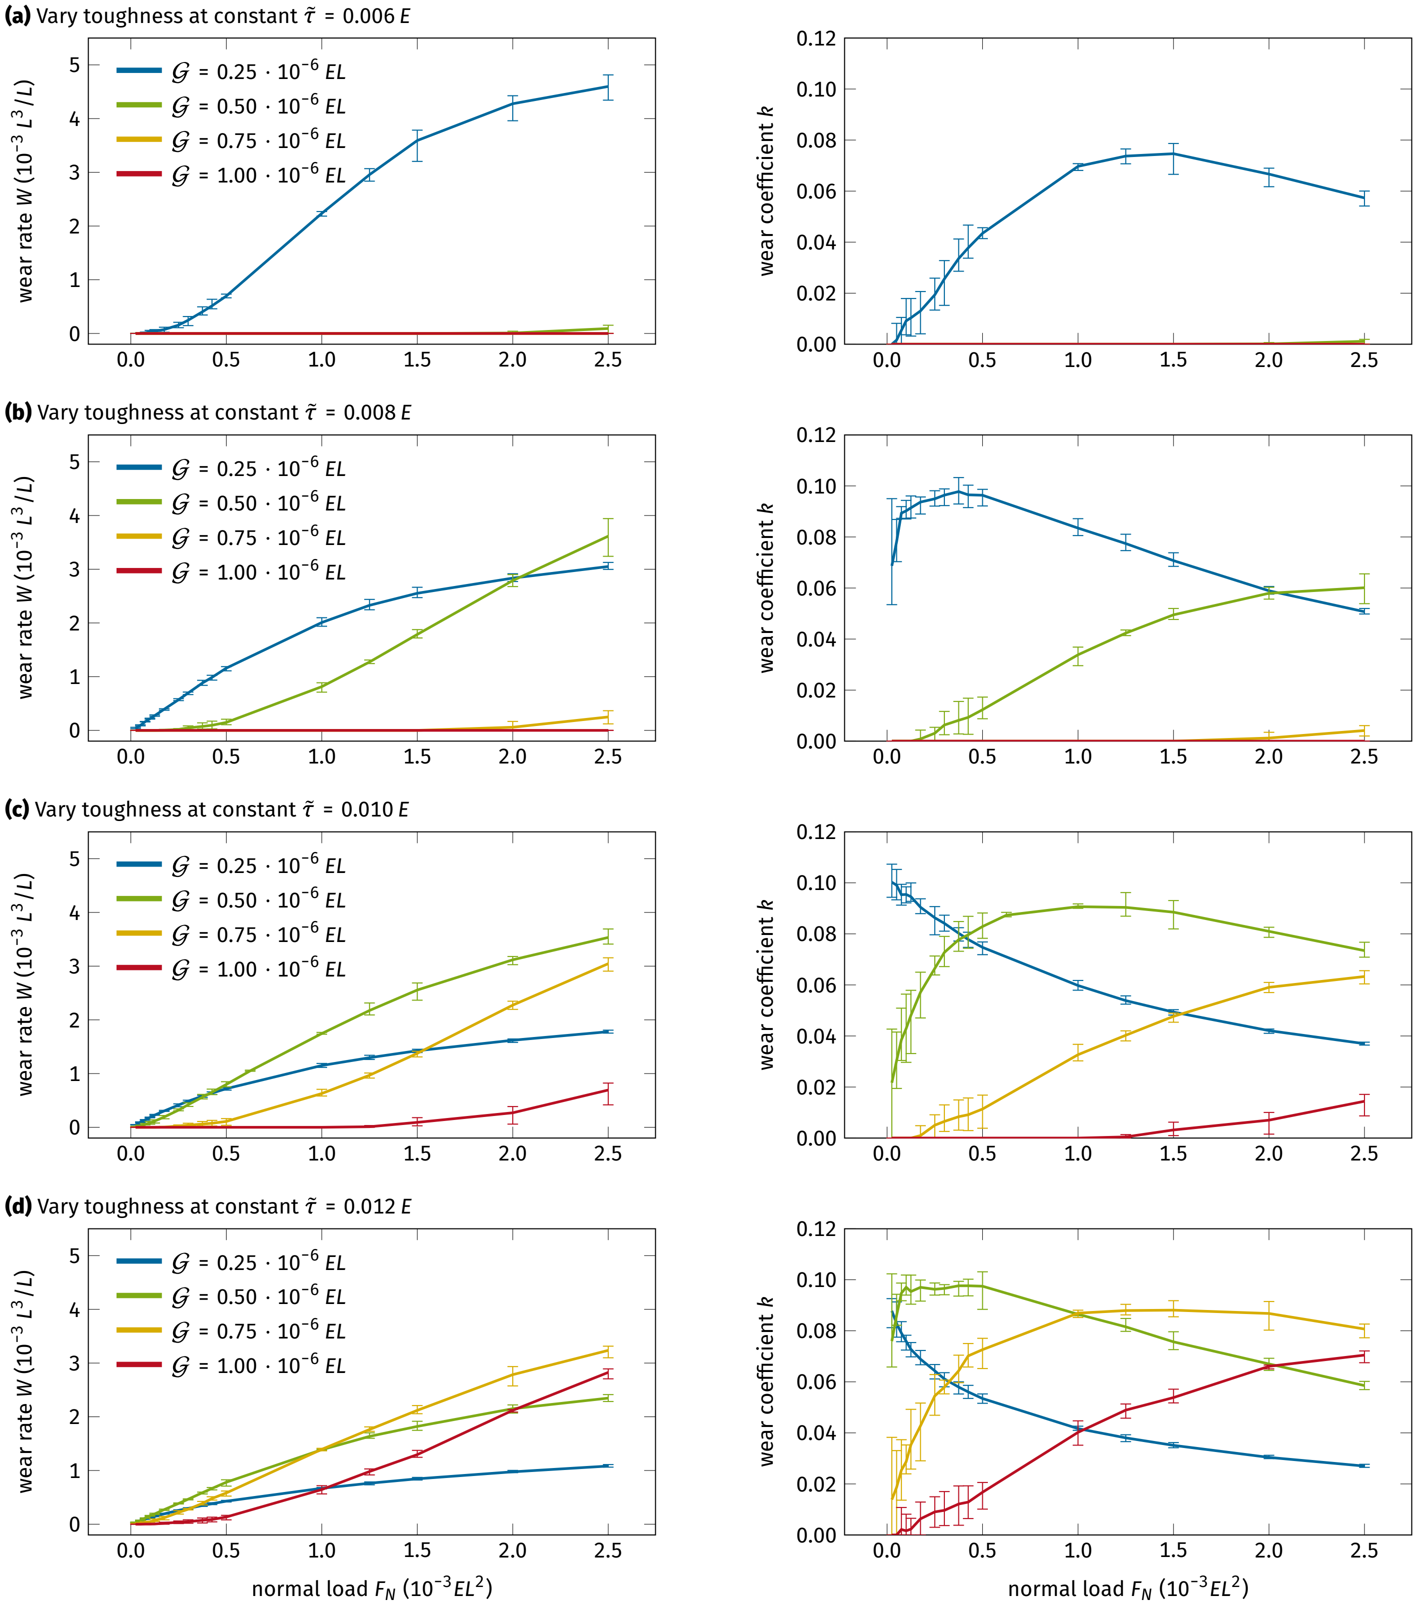


**Figure S.1:** Wear rates and wear coefficients predicted by our model for varying toughness at constant hardnesses. The data is the average of five simulations, the error bars indicate the minimum and maximum values.

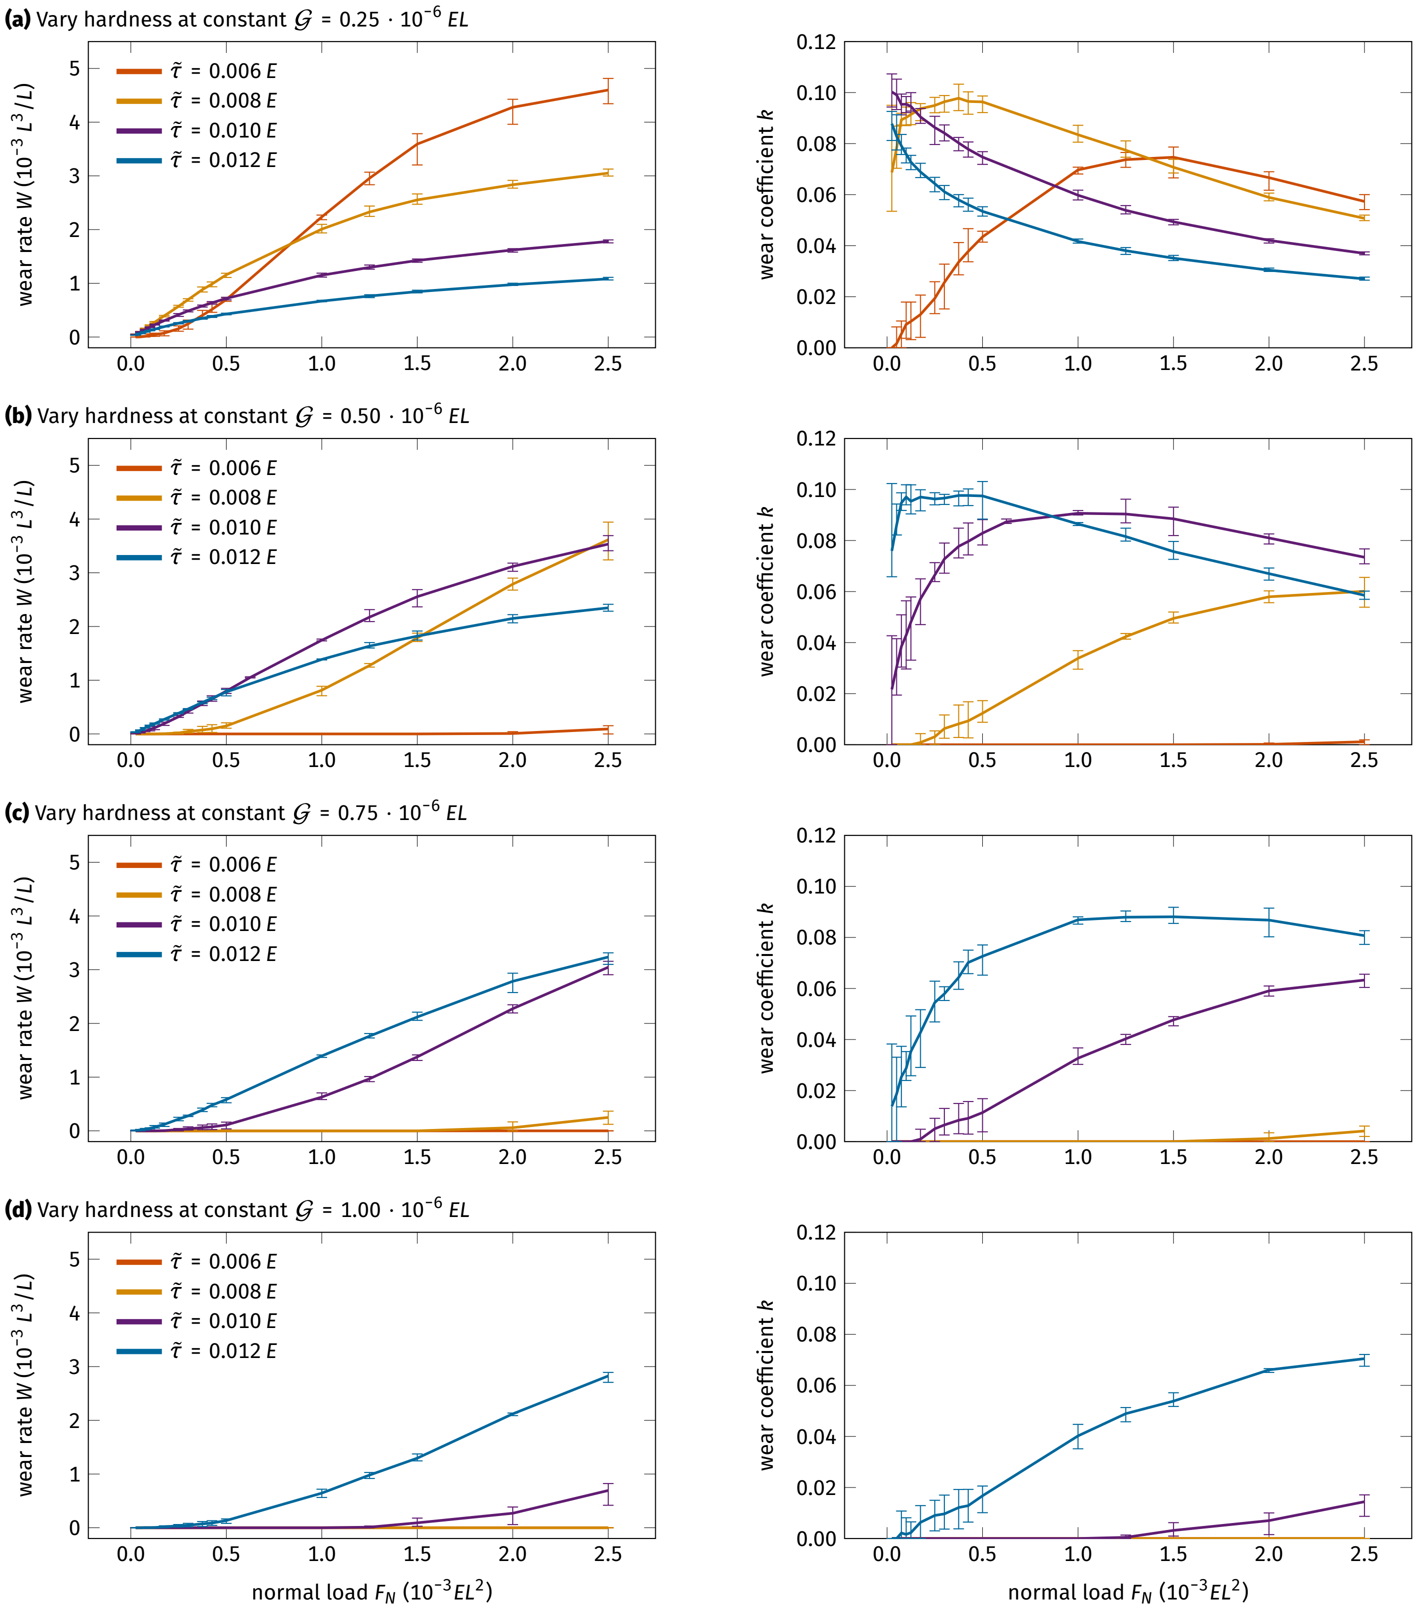


**Figure S.2:** Wear rates and wear coefficients predicted by our model for varying hardness at constant toughness. The data is the average of five simulations, the error bars indicate the minimum and maximum values.

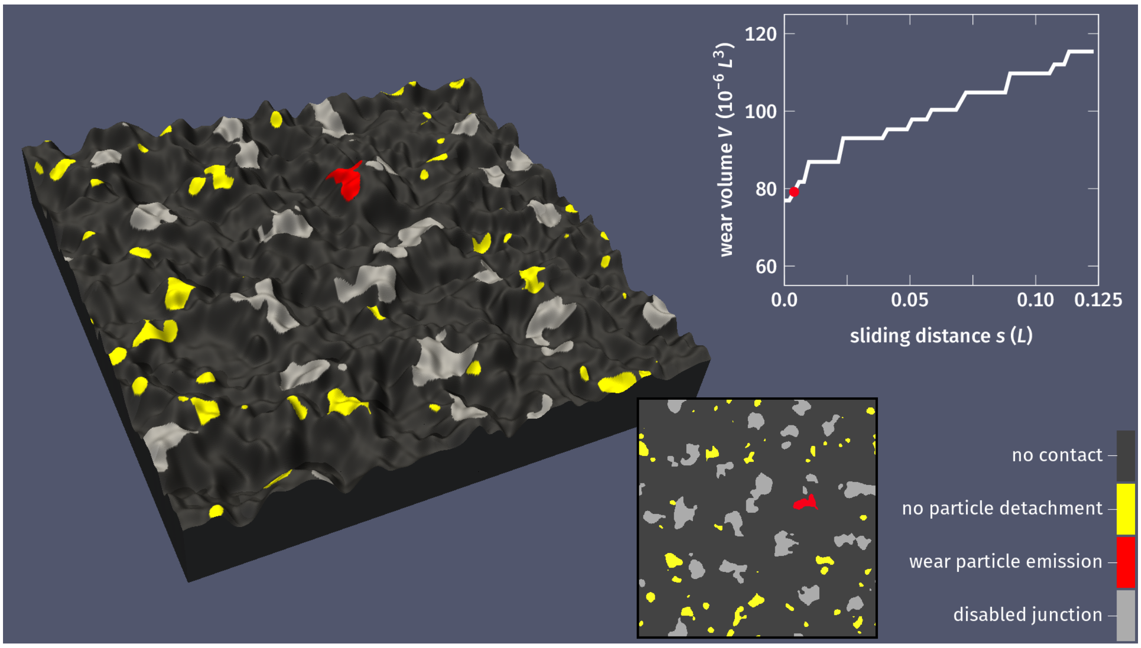


**Video 1:** Video of a smaller simulation with side length $0.25\,L$ discretized into $512 \times 512$ pixels, $\lambda_l = L/128$, $\lambda_u = L/16$, $H = 0.7$, $h_{\mathrm{RMS}} = 0.005\,L$, $\nu = 0.3$, $\tilde{\tau} = 0.006\,E$, $\mathcal{G} = 0.25 \cdot 10^{-6}\,EL$, where $L$ corresponds to the side length of the surfaces used in the main text. The normal load is $F_N = 0.25 \cdot 10^{-3}\,EL^2$. The simulation was made smaller to make the features of the model easier to see. On the left a 3D view of the bottom surface is shown, the contacting areas colored according to the wear behavior: no particle detachment (yellow), a wear particle is emitted at the present moment (red), or the junction has already emitted a particle in a previous step (gray). The smaller inset at the bottom shows the same as a top view. Filename: `video1-load_250e-6.mp4`.

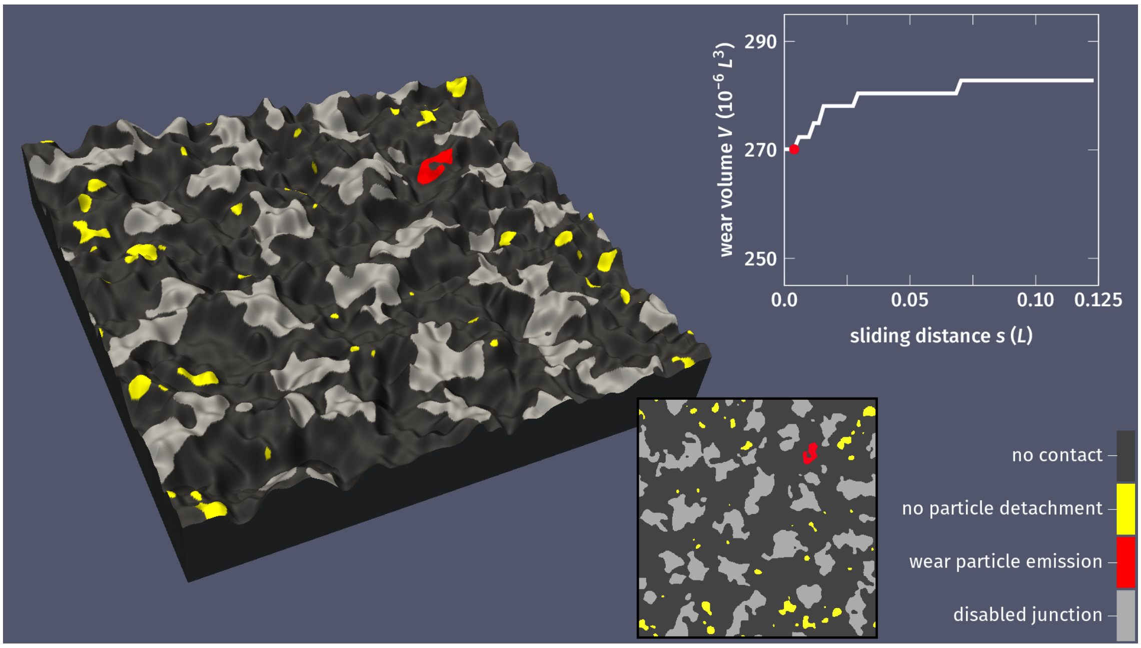


**Video 2:** The same as Video 1, but with a normal load of $F_N = 0.5 \cdot 10^{-3}\,EL^2$. Due to the merging of contact junctions, the wear rate is significantly lower than at smaller normal loads, indicating the limits of the model for high loads and small surfaces. Filename: `video2-load_500e-6.mp4`.
